# Supplementary material for: First-principles study on phase stability and physical properties of B-site ordered Nd$_{2}$FeCrO$_{6}$ double perovskite
Source: arXiv:2201.02341 source file (2022-01-07)
Supplement: Supplementary file 1 [file appendix1.tex]

\section{Supplementary Material} \label{sec:appendix}
    Here the ESI will be included.
